# Supplementary material for: Current-induced forces for nonadiabatic molecular dynamics
Source: arXiv:1803.05440 source file (2018-03-14)
Supplement: Supplementary file 1 [file supp4.pdf]

# Supplemental Material: Current-induced forces for nonadiabatic molecular dynamics


Feng Chen,[1] Kuniyuki Miwa,[2,3] and Michael Galperin[2,*]

[1]Department of Physics, University of California San Diego, La Jolla, CA 92093, USA
[2]Department of Chemistry & Biochemistry, University of California San Diego, La Jolla, CA 92093, USA
[3]Surface and Interface Science Laboratory, RIKEN, Wako, Saitama, 351-0198, Japan


## DERIVATION OF EQ. (23)

Here we derive the fluctuation-dissipation theorem (23).

Taking Fourier transform of $\gamma_{\alpha\beta}(t_1 - t_2)$ and evaluating integral in $x$ leads to two equivalent expressions corresponding to two lines in (22)

$$\gamma_{\alpha\beta}(E) = +i\int \frac{d\omega}{2\pi}\frac{J_{\alpha\beta}(\omega)}{E-\omega+i\delta}\frac{1-e^{-\beta\hbar\omega}}{\hbar\omega} \tag{S1}$$

$$= -i\int \frac{d\omega}{2\pi}\frac{J_{\alpha\beta}(\omega)}{-E-\omega+i\delta}\frac{1-e^{-\beta\hbar\omega}}{\hbar\omega} \tag{S2}$$

where

$$J_{\alpha\beta}(\omega) = \int d(t_1-t_2)e^{i\omega}(t_1-t_2)\big\langle\partial_\alpha \hat{H}_e(t_1)\,\partial_\beta \hat{H}_e(t_2)\big\rangle_c \tag{S3}$$

and where in the derivation of (S2) we used [1]

$$J_{\beta\alpha}(-\omega) = J_{\alpha\beta}(\omega)e^{-\beta\hbar\omega} \tag{S4}$$

Two equivalent expressions in (22) lead to $\gamma_{\alpha\beta}(t_1-t_2) = \gamma^*_{\alpha\beta}(t_1-t_2)$ and hence

$$\gamma^*_{\alpha\beta}(E) = \gamma_{\alpha\beta}(-E) \tag{S5}$$

Thus, using (S1) and (S2) and taking into account relation (S5) leads to

$$2\,\mathrm{Re}\,\gamma_{\alpha\beta}(E) \equiv \gamma_{\alpha\beta}(E) + \gamma_{\alpha\beta}(-E) = J_{\alpha\beta}(E)\frac{1-e^{-\beta E}}{E} \tag{S6}$$

Fourier transform of (13) is

$$\Pi_{\alpha\beta}(E) = \frac{1+e^{-\beta E}}{2}J_{\alpha\beta}(E) \tag{S7}$$

where we again used (S4). Finally, using (S6) in (S7) leads to (23).

## CONNECTION WITH RESULTS OF REF. 29

To detail the connection we consider non-interacting electronic Hamiltonian of Ref. 29

$$\hat{H}_M(\hat{q}) = \sum_{i,j}\left(H^0_{ij} + \sum_\alpha M^\alpha_{ij}\,\hat{q}_\alpha\right)\hat{c}^\dagger_i\hat{c}_j \tag{S8}$$

instead of general form (2) in (13) and (26). This leads to expressions for dissipation and fluctuation in terms of two-particle Green functions. Applying the Wick's theorem [3] immediately yields results of the work

$$\Pi^r_{\alpha\beta}(t_1,t_2) = i\theta(t_1-t_2)\,\mathrm{Tr}\big[M^\alpha G^<(t_1,t_2)M^\beta G^>(t_2,t_1) - M^\alpha G^>(t_1,t_2)M^\beta G^<(t_2,t_1)\big] \tag{S9}$$

$$\Pi_{\alpha\beta}(t_1,t_2) = \frac{1}{2}\mathrm{Tr}\big[M^\alpha G^>(t_1,t_2)M^\beta G^<(t_2,t_1) + M^\alpha G^<(t_1,t_2)M^\beta G^>(t_2,t_1)\big] \tag{S10}$$

Here trace is over molecular orbitals and $G^{>/<}$ are the greater/lesser projections of the single-particle Green function $G_{ij}(\tau_1,\tau_2) \equiv -i\langle T_c\,\hat{c}_i(\tau_1)\,\hat{c}^\dagger_j(\tau_2)\rangle$, friction tensor $\Pi^r_{\alpha\beta}(t_1,t_2)$ originates from (26), and evolution of electron creation and annihilation operators $\hat{c}^\dagger_j(\tau_2)$ and $\hat{c}_i(\tau_1)$ is governed by $\hat{H}^{(0)}_e$ of (24).

Figure S1 compares NEGF simulations of Ref. 29 (exact for the model; solid line, red) with the Hubbard NEGF results (applicable also in interacting systems; dashed line, blue) and generalized version of the Head-Gordon and Tully friction tensor [43] (dotted line, black) for several system-bath coupling strengths Γ.

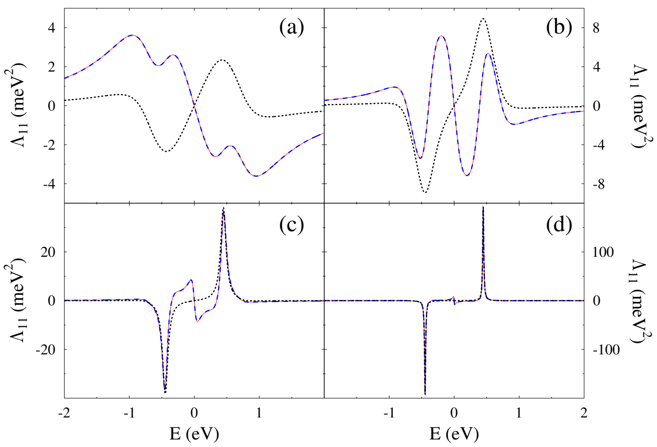


FIG. S1: Friction tensor $\Lambda_{11}(E)$ for the noninteracting junction model (Fig. 1). Simulations are performed for (a) $\Gamma = 0.5$ eV, (b) $\Gamma = 0.2$ eV, (c) $\Gamma = 0.05$ eV, and (d) $\Gamma = 0.01$ eV. Results of the NEGF calculation [29] (solid line, red) are compared with the Hubbard NEGF (dashed line, blue) and nonequilibrium generalization of the Head-Gordon and Tully electronic friction [43] (dotted line, black). Other parameters are as in Fig. 2.

## NON-CONDON EFFECTS IN CURRENT-INDUCED FORCES

Here we briefly discuss simulation of non-Condon effects in the friction tensor. Effective evaluation of nuclear coordinate dependence in the molecule-contacts coupling, Eq.(5), in interacting systems can utilize decoupling between molecular and contacts electronic degrees of freedom. For example, the non-Condon effects due to coupling-coupling correlation are given approximately by the following expressions, again involving only single-particle Hubbard Green functions (39)

$$\Pi^r_\alpha(t_1,t_2) = 2\,\mathrm{Im}\,\theta(t_1-t_2) \times \mathrm{Tr}\big[\Sigma^{(\alpha)\,>}(t_1,t_2)D^<(t_2,t_1) - \Sigma^{(\alpha)\,<}(t_1,t_2)D^>(t_2,t_1)\big] \tag{S11}$$

$$\Pi_{\alpha\beta}(t_1,t_2) = \mathrm{Tr}\big[\Sigma^{(\alpha\beta)\,>}(t_1,t_2)D^<(t_2,t_1) + \Sigma^{(\alpha\beta)\,<}(t_1,t_2)D^>(t_2,t_1)\big] \tag{S12}$$

Here trace is over single-electron transitions between many-body states of the molecule and $\Sigma^{(\alpha)\,>/<}$ and $\Sigma^{(\alpha\beta)\,>/<}$ are the greater/lesser projections of self-energies due to molecule-contacts coupling

$$\Sigma^{(\alpha)}_{S_1S_2,S_3S_4}(\tau_1,\tau_2) = \sum_k \partial_\alpha V_{S_1S_2,k}(Q)\, g_k(\tau_1,\tau_2)\, V_{k,S_3S_4}(Q) \tag{S13}$$

$$\Sigma^{(\alpha\beta)}_{S_1S_2,S_3S_4}(\tau_1,\tau_2) = \sum_k \partial_\alpha V_{S_1S_2,k}(Q)\, g_k(\tau_1,\tau_2)\, \partial_\beta V_{k,S_3S_4}(Q) \tag{S14}$$

and $g_k(\tau_1,\tau_2) \equiv -i\langle T_c\, \hat c_k(\tau_1)\, \hat c_k^\dagger(\tau_2)\rangle$ is Green function of free electrons in state $k$ of contacts. Similar evaluation of molecule-coupling cross terms will result in multi-time Hubbard correlation functions. Diagrammatic technique allows pretty accurate evaluation of the latter as well [4].

---

* Electronic address: `migalperin@ucsd.edu`

[1] D. Zubarev, V. Morozov, and G. Röpke, *Statistical Mechanics of Nonequilibrium Processes* (Akademie Verlag, Berlin, 1996).

[2] J.-T. Lü, M. Brandbyge, P. Hedegård, T. N. Todorov, and D. Dundas, Phys. Rev. B **85**, 245444 (2012).

[3] A. L. Fetter and J. D. Walecka, *Quantum Theory of Many-Particle Systems* (McGraw-Hill Book Company, 1971).

[4] K. Miwa, F. Chen, and M. Galperin, Sci. Rep. **7**, 9735 (2017).
